# Supplementary material for: Observation of a many-body-localized discrete time crystal with a programmable spin-based quantum simulator
Source: arXiv:2107.00736 ancillary file (2021-07-01)
Supplement: Supplementary file 1 [file SupplementaryMaterials.pdf]

# Supplementary Material: Observation of a many-body-localized discrete time crystal with a programmable spin-based quantum simulator

(Dated: June 24, 2021)

## I. EXPERIMENTAL SETUP

### A. Sample and NV center

The experiments are performed on a naturally occurring NV center using a home-built confocal microscope based on a 3.7 K cryostat (Montana Cryostation). The diamond was homoepitaxially grown using chemical vapor deposition and cleaved along the  $\langle 111 \rangle$  axis (Element Six). There is a natural abundance (1.1%) of  $^{13}\text{C}$ . The NV centre was selected on the absence of strongly coupled  $^{13}\text{C}$  spins ( $> 500$  kHz hyperfine coupling), but without any other criteria on the spin environment. An external magnetic field of  $B_z = 403.553$  G is applied along the NV-axis (the  $z$ -axis) using a permanent neodymium magnet, which is temperature stabilized using a feedback loop [1]. The field is aligned to within 0.1 degrees using a thermal echo sequence [2]. The NV electron spin has a dephasing time of  $T_2^* = 4.9(2)$   $\mu\text{s}$  and a spin echo time of  $T_2 = 1.182(5)$  ms, which can be extended to  $T_2^{\text{DD}} > 1$  s using dynamical decoupling [3]. The electron relaxation ( $T_1 > 1$  h) at this temperature is negligible [3]. We measure the NV electron spin state in a single shot using spin-selective optical readout [4]. The readout fidelities are 0.905(2) (0.986(2)) for the  $m_s = 0$  ( $m_s = -1$ ) state with an average fidelity of  $F = 0.946(1)$ . All measurements are corrected for readout in order to provide a best estimate for the actual state.

### B. Microwave pulses

We apply microwave pulses to drive the NV electron spin transition  $m_s = 0 \leftrightarrow m_s = -1$  at 1.746666(3) GHz using single-sideband modulation. IQ signals are generated at 250 MHz using an AWG (Tektronix 5014C) and upconverted using a vector RF source (Rohde & Schwarz SGS100A). The output of this source is then amplified (AR 25S1G6). Microwave amplifier noise is suppressed by 40 dB using a fast microwave switch (TriQuint TGS2355-SM). Video leakage noise generated by the switch is filtered with a high pass filter. For the PulsePol sequence used for initialization of the simulator (section VI), square pulse envelopes are used with duration 30 ns (15 ns) for a  $\pi$  ( $\pi/2$ ) pulse. During dynamical decoupling gates for nuclear-spin readout (section V), Hermite pulse envelopes [5, 6] are used to obtain high-fidelity rotations of the electron spin independent of the  $^{14}\text{N}$  nuclear spin state, with peak Rabi frequencies of 35 MHz (23 MHz) for a  $\pi$  ( $\pi/2$ ) pulse. Pulse errors during dynamical decoupling are mitigated using the XY8 scheme [7].

### C. Radio-frequency pulses

We apply radio-frequency (RF) pulses in the frequency range 400 – 500 kHz (see Table S1) to directly and selectively drive the  $^{13}\text{C}$  spins. To prepare initial states of the form  $|m_j\rangle^{\otimes N}$ ,  $m_j \in \{\uparrow, \downarrow\}$ , and for the rotations used in the nuclear-nuclear readout method (section V), we use single-frequency pulses with an error-function envelope [1]. For the  $x$ -rotations in the Floquet sequence, and the global basis rotations used to initialize the states  $|++++\rangle$  (Fig. 2B of the main text) and  $[\cos(\pi/8)|\uparrow\rangle + \sin(\pi/8)|\downarrow\rangle]^{\otimes L}$  (Figs. 3F,G of the main text), and to read out  $\langle\sigma_j^x\rangle / \langle\sigma_j^y\rangle$ , we use multi-frequency pulses. This allows us to rotate all 9 spins in the 1D chain simultaneously and independently of other spins in the environment, which is crucial for realising the Floquet sequence in these experiments. To reduce crosstalk between spins, we use a  $\sin^2$  pulse envelope for the multi-frequency pulses. The waveform for a pulse containing  $L$  frequency components is therefore given by

$$V(t) = \sin^2\left(\frac{\pi t}{t_p}\right) \sum_j^L V_j \cos\left(2\pi f_j(t - \frac{t_p}{2}) + \phi_j\right), \quad (\text{S1})$$

where  $t_p$  is the pulse length,  $V_j$ ,  $f_j$  and  $\phi_j$  are the amplitude, frequency and phase of frequency component  $j$ , respectively, and  $t$  runs from 0 to  $t_p$ .

In order to generate the multi-frequency pulses with sufficient power, we amplify the signal from an AWG (Tektronix 5014C) using an RF amplifier (Analog Devices ADA4870, gain +12 dB), and apply filtering to reduce additional noise

on the signal (3rd-order Butterworth high-pass filter, 52 kHz, and 7th-order linear-phase low-pass filter, 850 kHz, both home-built). Additionally, we stagger the phases  $\phi_j$  of each pulse to ensure that the frequency components do not constructively interfere at the center of the  $\sin^2$  pulse envelope.

Applying multiple frequency components to the nuclear spins simultaneously can cause AC Stark shifts if two spins are close in frequency. To minimize coherent pulse errors from such shifts, we iteratively calibrate the pulse parameters for each spin (frequency and amplitude). The resulting calibrated frequency components for each spin are given in Table S1.

## II. DERIVATION OF $H$ AND $U_F$

### A. Interaction Hamiltonian

The Hamiltonian of the ground-state NV electron spin coupled to a bath of interacting  $^{13}\text{C}$  nuclear spins is given by

$$H = \Delta_{\text{ZFS}}(S^z)^2 + \gamma_e B_z S^z + \sum_j \gamma_c \vec{B} \cdot \vec{I}_j + \sum_j \vec{S} \cdot \mathbf{A}_j \cdot \vec{I}_j + \sum_{j < k} \vec{I}_j \cdot \mathbf{C}_{jk} \cdot \vec{I}_k, \quad (\text{S2})$$

where  $\Delta_{\text{ZFS}}$  is the zero-field splitting,  $\gamma_e$  ( $\gamma_c$ ) is the electron ( $^{13}\text{C}$  nuclear) gyromagnetic ratio,  $B_z$  is the externally applied global magnetic field along the  $z$ -axis,  $\mathbf{A}_j$  is the electron- $^{13}\text{C}$  hyperfine tensor for nuclear spin  $j$  and  $\mathbf{C}_{jk}$  is the  $^{13}\text{C}$ - $^{13}\text{C}$  dipole-dipole coupling tensor between nuclear spins  $j$  and  $k$ . Here  $\vec{S} = (S^x, S^y, S^z)$  and  $\vec{I}_j = (I_j^x, I_j^y, I_j^z)$  are the spin vectors for the electron and nuclear spins, respectively, where  $S^\alpha$  are the spin-1 matrices representing the electron spin ground state levels  $m_s = \{0, \pm 1\}$  and  $I_j^\alpha = \sigma_j^\alpha/2$ , where  $\sigma_j^\alpha$  are the Pauli spin matrices. In the experiments described in the main text, the electron spin is prepared in the  $m_s = -1$  eigenstate for the duration of the quantum simulation part of the sequence ( $U_F$  in Fig. 1B of the main text). We therefore only need to consider the nuclear spin Hamiltonian for the  $m_s = -1$  state, given by

$$H_{-1} = \sum_j \left[ (\gamma_c B_z - A_j^\parallel) I_j^z - A_j^\perp (\cos(\varphi_j^\perp) I_j^x + \sin(\varphi_j^\perp) I_j^y) \right] + \sum_{j < k} \vec{I}_j \cdot \mathbf{C}_{jk} \cdot \vec{I}_k, \quad (\text{S3})$$

where  $A_j^\parallel = A_j^{zz}$  is the parallel hyperfine component,  $A_j^\perp = \sqrt{(A_j^{zx})^2 + (A_j^{zy})^2}$  is the perpendicular hyperfine magnitude and  $\varphi_j^\perp$  is the perpendicular hyperfine azimuthal angle. Other hyperfine interaction terms have been neglected in the secular approximation. This Hamiltonian is used for the numerical simulations presented in Fig. 2 of the main text. The hyperfine and nuclear-nuclear interactions for the 9 spins are given in Tables S1 and S2, while the azimuthal angles  $\varphi_\perp^j$  are approximated from the known spatial angles relative to the position of the vacancy lattice site<sup>1</sup> (Table S1).

In our experiments we apply a strong magnetic field of  $B_z \sim 403$  G. In this case, we can further simplify  $H_{-1}$  by using the fact that  $(\gamma_c B_z - A_j^\parallel) \gg A_j^\perp$  and  $|A_j^\parallel - A_k^\parallel| \gg C_{jk}^{zz}$  for all  $j, k$ . This allows us to neglect non-secular terms and therefore obtain the interaction Hamiltonian  $H_{\text{int}}$  presented in Eq. 1 of the main text, given by

$$H_{-1} \approx H_{\text{int}} = \sum_j (B + h_j) \sigma_j^z + \sum_{j < k} J_{jk} \sigma_j^z \sigma_k^z, \quad (\text{S4})$$

where  $B + h_j = \frac{1}{2} \sqrt{(\gamma_c B_z - A_j^\parallel)^2 + (A_j^\perp)^2}$  and  $J_{jk} = C_{jk}^{zz}/4$ . For  $B + h_j$  we have here included the contribution from  $A_j^\perp$  to the precession frequency [8]. This Hamiltonian is used for the numerical simulations presented in sections VII and VIII.

---

<sup>1</sup> Note that these angles are only equal under the approximation that the electron is a point dipole located at the vacancy, and therefore the actual hyperfine azimuthal angles may differ due to the finite size and shape of the electron wavefunction.

## B. Spin rotations

As described in section IC, the spin rotations in the Floquet sequence are implemented using multi-frequency rf pulses. With a general time-dependent voltage  $V(t)$ , the nuclear-spin Hamiltonian has an additional term

$$H_{\text{rf}}(t) = \sum_j \Omega(t) \sigma_j^x, \quad (\text{S5})$$

where  $\Omega(t) = \gamma_c \beta V(t)$  with  $\beta$  being a conversion factor from applied voltage to magnetic field at the NV center. We assume that the field is polarized in the  $x$ -direction<sup>2</sup>. Together with Eq. S4, this term gives Eq. 1 of the main text,  $H(t) = H_{\text{int}} + H_{\text{rf}}(t)$ .

We apply multi-frequency pulses of the form given in Eq. S1. For the simulations presented in Fig. 2 of the main text, the unitary evolution during the pulses is calculated by numerically integrating the time-dependent Hamiltonian  $H_{-1} + H_{\text{rf}}(t)$ , with  $V(t)$  given by Eq. S1, using the QuTiP Python package [9]. To arrive at the Floquet operator  $U_F$ , we can simplify  $H(t)$  under the approximation that the spin-spin interactions can be neglected during the pulse, which is valid in the regime  $\Omega_j \gg J_{jk}$ , where  $\Omega_j = \gamma_c \beta V_j$ . In this case, after transforming to the interaction picture with respect to  $H_0 = \sum_j (B + h_j) \sigma_j^z$  and setting each frequency component in  $V(t)$  (Eq. S1) equal to one of the spin precession frequencies ( $2\pi f_j = 2(B + h_j)$ ), the Hamiltonian becomes

$$\begin{aligned} H'(t) &= e^{iH_0 t} H(t) e^{-iH_0 t} - H_0 \\ &= \sin^2 \left( \frac{\pi t}{t_p} \right) \sum_j \frac{\Omega_j}{2} (\cos(\phi'_j) \sigma_j^x + \sin(\phi'_j) \sigma_j^y), \end{aligned} \quad (\text{S6})$$

where  $\phi'_j = \phi_j - (B + h_j)t_p$  and we have neglected off-resonant terms. Since  $[H'(t_1), H'(t_2)] = 0$ , we can use the fact that

$$\int_0^{t_p} \sin^2 \left( \frac{\pi t}{t_p} \right) dt = \frac{t_p}{2}, \quad (\text{S7})$$

to calculate the unitary operator at  $t = t_p$  in the rotating frame, given by

$$\begin{aligned} U'(t_p) &= \exp \left( -i \int_0^{t_p} H'(t) dt \right) \\ &= \exp \left( i \frac{t_p}{2} H_0 \right) \cdot \exp \left( -i \frac{t_p}{2} \sum_j \frac{\Omega_j}{2} (\cos(\phi_j) \sigma_j^x + \sin(\phi_j) \sigma_j^y) \right) \cdot \exp \left( -i \frac{t_p}{2} H_0 \right), \end{aligned} \quad (\text{S8})$$

where in the second line we have used the identity

$$e^{-i\theta(\cos(\phi_0 + \phi_1)\sigma^x + \sin(\phi_0 + \phi_1)\sigma^y)} = e^{-i\phi_1\sigma^z/2} e^{-i\theta(\cos(\phi_0)\sigma^x + \sin(\phi_0)\sigma^y)} e^{i\phi_1\sigma^z/2}. \quad (\text{S9})$$

Finally, we can revert to the lab frame, giving

$$\begin{aligned} U(t_p) &= e^{-iH_0 t_p} U'(t_p) \\ &= \exp \left( -i \frac{t_p}{2} H_0 \right) \cdot \exp \left( -i \sum_j \frac{\theta_j}{2} (\cos(\phi_j) \sigma_j^x + \sin(\phi_j) \sigma_j^y) \right) \cdot \exp \left( -i \frac{t_p}{2} H_0 \right). \end{aligned} \quad (\text{S10})$$

---

<sup>2</sup> In reality the polarization is not known, however field components in the  $z$ -direction will cancel in the rotating wave approximation as long as they oscillate sufficiently fast, and therefore the only effect would be a reduction in the experimentally determined parameter  $\beta$  for all spins. Field components in the  $y$ -direction will add a global phase shift, which can be neglected without loss of generality for the experiments described in this work.

The effect of the multi-frequency pulse under these approximations is therefore equivalent to instantaneous rotations of each spin by an angle  $\theta_j = \Omega_j t_p/2$  around an axis at angle  $\phi_j$  in the  $x - y$  plane, between two periods of free precession under the Hamiltonian  $H_0$  for time  $t_p/2$ .

For short pulse times and setting  $\phi_j = 0$  and  $\theta_j = \theta$ , we can approximate that  $U(t_p) \approx U_x(\theta) = \exp(-i\theta \sum_j^L \sigma_j^x/2)$ , as given in the main text. Combining with  $U_{\text{int}}(\tau) = \exp(-iH_{\text{int}}\tau)$ , we therefore arrive at the ideal Floquet sequence  $U_F = [U_{\text{int}}(\tau) \cdot U_x(\theta) \cdot U_{\text{int}}(\tau)]^N$ .

### C. Effective Hamiltonian

For  $\theta = \pi - \epsilon$ , the Floquet sequence unitary operator over two periods is given by

$$\begin{aligned} e^{-i2\tau H_{\text{eff}}} &= U_F^2 = U_{\text{int}}(\tau) \cdot U_x(\pi - \epsilon) \cdot U_{\text{int}}(2\tau) \cdot U_x(\pi - \epsilon) \cdot U_{\text{int}}(\tau) \\ &= U_0(\tau) \cdot U_{zz}(\tau) \cdot U_x(-\epsilon) \cdot X \cdot U_0(2\tau) \cdot U_{zz}(2\tau) \cdot X \cdot U_x(-\epsilon) \cdot U_0(\tau) \cdot U_{zz}(\tau) \\ &= U_0(\tau) \cdot U_{zz}(\tau) \cdot U_x(-\epsilon) \cdot U_0(-2\tau) \cdot U_{zz}(2\tau) \cdot U_x(-\epsilon) \cdot U_0(\tau) \cdot U_{zz}(\tau), \end{aligned} \quad (\text{S11})$$

where  $X = (\sigma_j^x)^{\otimes L}$  is a global  $x$ -rotation of the spins and we have split  $U_{\text{int}}(\tau)$  into single-spin terms  $U_0(\tau) = \exp(-i\tau \sum_j (B + h_j)\sigma_j^z)$  and pairwise interactions  $U_{zz}(\tau) = \exp(-i\tau \sum_{j < k} J_{jk} \sigma_j^z \sigma_k^z)$ . To leading order in  $\epsilon$  (valid for  $\epsilon \ll \pi$ ), the effective Hamiltonian is given by the time-average of the exponents in Eq. S11 [10, 11], given by

$$\begin{aligned} H_{\text{eff}} &\approx \frac{1}{4\tau} \left[ 4\tau \sum_{j < k} J_{jk} \sigma_j^z \sigma_k^z - \epsilon \sum_j \sigma_j^x \right] \\ &= \sum_{j < k} J_{jk} \sigma_j^z \sigma_k^z - \frac{\epsilon}{4\tau} \sum_j \sigma_j^x. \end{aligned} \quad (\text{S12})$$

This effective Hamiltonian is used to calculate the energy density  $\mathcal{E} = \langle H_{\text{eff}} \rangle / J_0 L$  for different initial product states in the diagram in Fig. 4E of the main text. The wide range of energy densities serves to illustrate the variety of initial states considered, despite  $H_{\text{eff}}$  not being a conserved quantity of the dynamics.

### D. $U_F$ without interactions

In Figs. 2B and 3B,C of the main text, we apply the Floquet sequence with the interactions turned off. This is achieved by individually applying the sequence to each spin in turn. For  $\theta \sim \pi$ , this decouples each targeted spin from the others and is therefore equivalent to evolving under  $U_F$  with  $J_{jk} = 0$  for all  $j, k$ .

## III. PROGRAMMING THE 1D CHAIN

### A. Identifying the chain

As discussed in the main text, many-body localization (MBL) is only stabilized if the spin-spin interactions  $J_{jk}$  are sufficiently short-ranged. We have a system of nuclear spins randomly positioned in 3 dimensional space, that interact through dipolar interactions which exhibit a power-law scaling  $1/r^3$ . This power-law exponent,  $\alpha = 3$ , is thus equal to the system dimensionality,  $d = 3$ , whereas MBL is compatible with  $\alpha > 2d$  [12, 13].

To resolve this challenge, we use a decoupling sequence to isolate a subset of spins which have a smaller effective dimensionality. In previous work, we characterized 27 individual  $^{13}\text{C}$  spins surrounding this NV centre [2]: their coupling matrix of 351 mutual interaction strengths are known. In principle, complex decoupling sequences can be used to realize any type of effective coupling matrix. Here, we consider a sequence that decouples 9 spins from the other spins, and look for a combination of spins that naturally forms an effective 1D chain. We thus perform a numerical search for a suitable effective 1D system (a spin chain) using those known parameters.

Starting from each of the 27 spins, we consider links to any other spin in the system, and accept all cases where the nearest-neighbor coupling exceeds  $|J_{jk}| = 2.5 \text{ Hz}$ . We then try to add a third spin, which must again exhibit a

| Spin | $A_{\parallel}$ (kHz) | $A_{\perp}$ (kHz) | $f_{-1,j}$ (Hz) |
|------|-----------------------|-------------------|-----------------|
| 1    | -5.62(1)              | 5(2)              | 437665(12)      |
| 2    | -19.815(3)            | 5.3(5)            | 451816(5)       |
| 3    | -13.961(3)            | 9(1)              | 445960(6)       |
| 4    | -4.66(3)              | 7(4)              | 436606(8)       |
| 5    | 17.643(1)             | 8.6(2)            | 414367(3)       |
| 6    | -11.346(2)            | 59.21(3)          | 447450(11)      |
| 7    | -14.07(2)             | 13(1)             | 446627(7)       |
| 8    | -48.58(2)             | 9(2)              | 480667(7)       |
| 9    | -9.79(2)              | 5(4)              | 441763(17)      |

TABLE S1. Measured parameters for the 9  $^{13}\text{C}$  nuclear spins used in this work.  $A_{\parallel}$  ( $A_{\perp}$ ): Parallel (perpendicular) hyperfine couplings.  $f_{-1,j}$ : Calibrated frequency components for each spin for the 9-frequency pulse (Eq. S1).

| Spin | $x$ (nm) | $y$ (nm) | $z$ (nm) |   | 1        | 2        | 3        | 4       | 5        | 6        | 7        | 8        | 9        |
|------|----------|----------|----------|---|----------|----------|----------|---------|----------|----------|----------|----------|----------|
| 1    | 0.000    | 0.000    | 0.000    | 1 | -        | -10.8(2) | -0.52    | 0.28    | -0.19    | -0.20    | -0.12    | -0.19    | -0.10    |
| 2    | -0.126   | -0.073   | 0.669    | 2 | -10.8(2) | -        | 4.44(4)  | 1.0(1)  | -0.08    | -0.39    | -0.23    | -0.4(1)  | -0.19    |
| 3    | -0.504   | 0.582    | 0.669    | 3 | -0.52    | 4.44(4)  | -        | 12.3(2) | -1.8(2)  | -0.95(5) | -0.31    | -0.33    | -0.17    |
| 4    | -0.378   | 1.092    | 0.618    | 4 | 0.28     | 1.0(1)   | 12.3(2)  | -       | -2.5(5)  | -0.60    | -0.22    | -0.20    | -0.14    |
| 5    | -0.631   | 1.092    | 1.699    | 5 | -0.19    | -0.08    | -1.8(2)  | -2.5(5) | -        | -3.88(2) | -0.90    | -0.18    | -0.30    |
| 6    | -0.631   | 0.655    | 2.317    | 6 | -0.20    | -0.39    | -0.95(5) | -0.60   | -3.88(2) | -        | -9.48(5) | 1.2(4)   | -0.4(1)  |
| 7    | -0.757   | 0.437    | 2.934    | 7 | -0.12    | -0.23    | -0.31    | -0.22   | -0.90    | -9.48(5) | -        | 3.5(5)   | 1.25     |
| 8    | -0.126   | 0.073    | 2.729    | 8 | -0.19    | -0.4(1)  | -0.33    | -0.20   | -0.18    | 1.2(4)   | 3.5(5)   | -        | -6.32(2) |
| 9    | 0.126    | 0.364    | 3.295    | 9 | -0.10    | -0.19    | -0.17    | -0.14   | -0.30    | -0.4(1)  | 1.25     | -6.32(2) | -        |

TABLE S2. Coordinates (left, relative to Spin 1) and spin-spin interactions  $J_{jk}$  (right, in Hz) for the 9 spins, taken from Abobeih et al. [2]. Interactions given with uncertainties were directly measured for the electron state  $m_s = -1$ , while values without uncertainties are calculated from the coordinates using Eq. S13.

nearest-neighbor coupling  $> 2.5$  Hz to either end of the chain, but additionally must not have any non-nearest-neighbor coupling  $> 2$  Hz. We iteratively add further spins which satisfy these requirements to identify a suitable spin chain. For the 9-spin chain we selected, we fit an average power-law exponent of  $\alpha = 2.5(1)$  (Fig. 1D of the main text).

## B. 1D chain spin parameters

Table S1 gives the parameters for the 9  $^{13}\text{C}$  spins used in this work. The first two columns give the electron-nuclear hyperfine couplings  $A_{\parallel}$  and  $A_{\perp}$  (Abobeih et al. [2]), which are extracted from the measured precession frequencies for different NV electron  $m_s$  states. The final column gives the calibrated frequency components used for the 9-frequency pulse (Eq. S1), which includes small frequency shifts due to couplings to other polarized spins and Stark shifts from off-resonant frequency components.

Table S2 gives the coordinates and spin-spin interactions  $J_{jk}$  for the 9 spins (Abobeih et al. [2]). Interactions with uncertainties given in parentheses are measured values for the NV electron state  $m_s = -1$ . Interactions shown without uncertainties were not directly measured, but can be calculated from the known spin coordinates [2] using the dipole-dipole formula, given by [14]

$$J_{jk} = \frac{C_{jk}^{zz}}{4} = \frac{C_0}{4\Delta r_{jk}^3} \left( 1 - \frac{3(z_j - z_k)^2}{\Delta r_{jk}^2} \right), \quad (\text{S13})$$

where  $\Delta r_{jk} = \sqrt{(x_j - x_k)^2 + (y_j - y_k)^2 + (z_j - z_k)^2}$ ,  $C_0 = \mu_0 \gamma_c^2 \hbar / 4\pi$ ,  $\mu_0$  is the permeability of free space, and  $\hbar$  is the reduced Planck constant.

## IV. ADDITIONAL DATA

Fig. S1 shows individual spin magnetization data underlying Figs. 3B,C in the main text, as well as additional datasets for  $\tau = 7.5$  ms. Fig. S2 shows the underlying data for Figs. 3F,G of the main text.

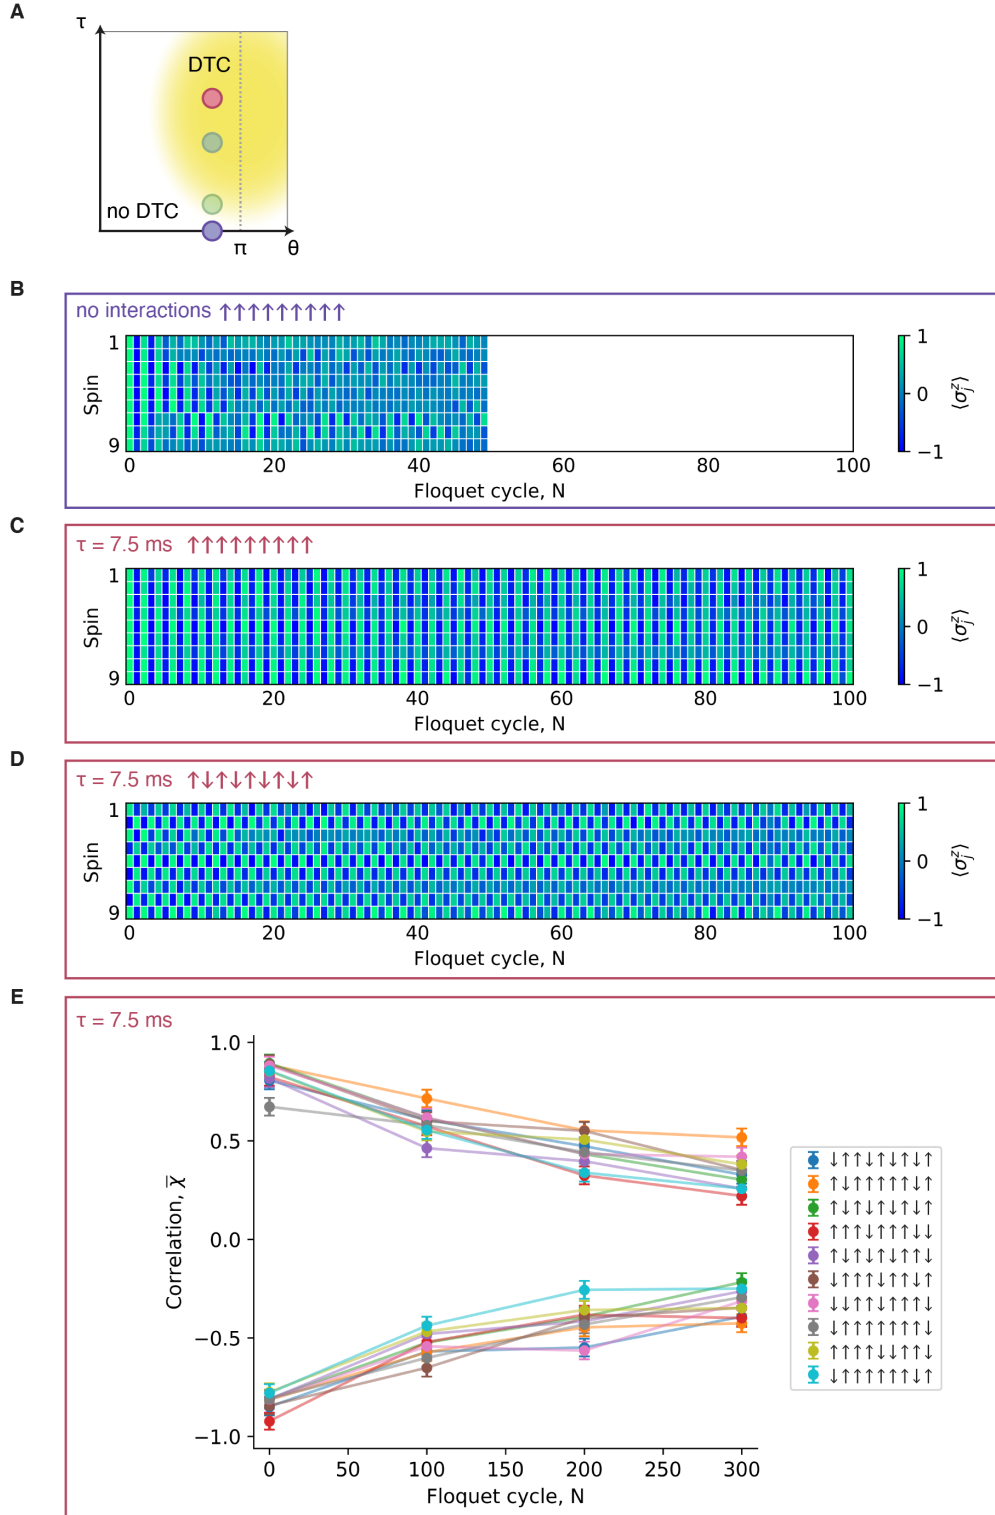

FIG. S1. **Additional DTC data.** Additional data showing individual spin magnetizations for different parameters  $\{\tau, \theta\}$ . (A) Phase diagram as shown in Fig. 3A of the main text, with an additional point shown (red,  $\tau = 7.5$  ms). (B) Individual spin results underlying the averaged plot shown in Figs. 3B, C of the main text for the case of no interactions (see section IID). (C-E) Additional datasets for  $\tau = 7.5$  ms (red point in (A)) for an initial polarized state (C), Néel state (D) and 10 of the initial states measured in Fig. 4D of the main text (E).

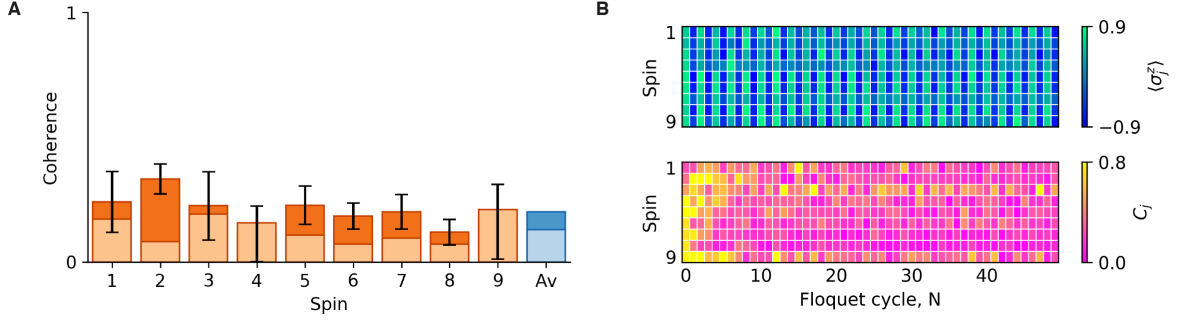

FIG. S2. **Individual spin data for Figs. 3F,G** (A) Measured coherence for each spin after preparing the state  $|\uparrow\uparrow\uparrow\uparrow\uparrow\uparrow\uparrow\uparrow\rangle$  (dark colored bars). The light shaded bars indicate the contribution from shot noise in the underlying measurements of  $\langle \sigma_j^x \rangle$  and  $\langle \sigma_j^y \rangle$ . The residual measured coherence is likely due to pulse errors in the  $\pi/2$  basis rotations. The blue bar shows the average of the orange bars over all spins. The dark blue bar is used to indicate a baseline in Fig. 3G in the main text. (B) Individual spin magnetizations (top) and coherences (bottom) after preparing the superposition state  $[\cos(\pi/8)|\uparrow\rangle + \sin(\pi/8)|\downarrow\rangle]^{\otimes 9}$ .

## V. READOUT OF THE FULL NUCLEAR-SPIN CHAIN

One of the key requirements for the experiments presented in this work is the ability to read out all individual spins within an interacting system. We develop a readout scheme in which some of the nuclear spins are directly read out through the NV electron spin, while other, not directly accessible, nuclear spins are first mapped to other nuclear spins that are accessible.

In previous work utilising  $^{13}\text{C}$  spins in diamond [1, 8], single-spin readout was achieved via dynamical decoupling sequences utilising individual electron-nuclear hyperfine interactions. However, these approaches require that the interactions are simultaneously strong (enabling fast, high fidelity gates), and spectrally heterogeneous (avoiding unwanted entanglement with non-targeted spins). This requirement is not generically met when considering larger nuclear spin systems, where some spins are only weakly coupled to the NV center. To overcome this challenge, we developed a new technique to read out nuclear spins that are more weakly coupled to the NV center electron spin, leveraging our knowledge of the spatial environment of the spin system and of the nuclear-nuclear couplings [2]. In particular, we isolate individual nuclear-nuclear interactions which can be used to map the state of a weaker coupled ‘target’ nuclear spin to a stronger coupled ‘probe’ nuclear spin. The stronger hyperfine interaction between the probe spin and the NV centre then enables readout using previously established techniques [1].

### A. Nuclear-nuclear readout

The desired quantum circuit to map the state from one nuclear spin to another is shown in Fig. 1B of the main text. Both the Hadamard and controlled-phase gates are not native to our system and must be compiled from native operations. Fig. S3A shows the compilation of the circuit replacing the Hadamard gates by native single qubit rotations. In Fig. S3B we show the compilation of the controlled-phase gate. The central feature is the ‘interaction’ block, where we interleave two periods of free evolution with concurrent spin-echo pulses applied to the target and probe spins (spin-echo double-resonance, SEDOR), with the electron spin in the state  $m_s = -1$ . These echo pulses serve to decouple the target and probe from all other spins while preserving their mutual interaction [2]. Under this condition, we can neglect the presence of other nuclear spins. From Eq. S4, we have

$$H_{-1} \approx H_{\text{int}} = (B + h_t)\sigma_t^z + (B + h_p)\sigma_p^z + J_{tp}\sigma_t^z\sigma_p^z, \quad (\text{S14})$$

with the parameters defined after Eq. S4. The subscripts  $t$  and  $p$  denote the target and probe spins, respectively. The unitary evolution during the interaction block is given by

$$U_{\text{SEDOR}}(\tau) = U_{\text{int}}(\tau) \cdot R_p^x(\pi) \cdot R_t^x(\pi) \cdot U_{\text{int}}(\tau). \quad (\text{S15})$$

Here,  $U_{\text{int}}(\tau) = \exp(-iH_{\text{int}}\tau)$  and  $R_j^\phi(\theta) = e^{-i\theta(\cos(\phi)\sigma_j^x + \sin(\phi)\sigma_j^y)/2}$  is a rotation of spin  $j$  by an angle  $\theta$  around an axis  $\phi$ . In the case that  $\tau = \tau_{\text{RO}} \equiv \pi/(8J_{tp})$ , this block realizes a maximally-entangling operation.

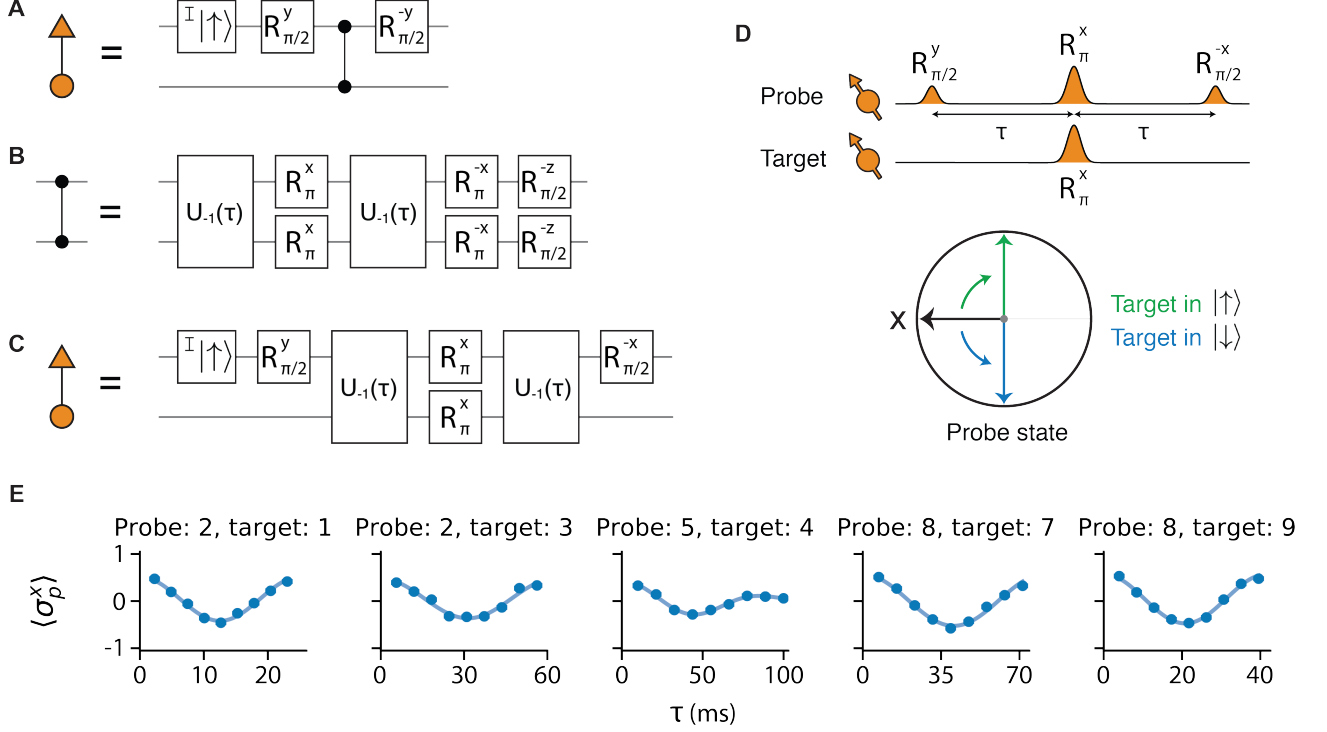

FIG. S3. **Nuclear-nuclear readout.** (A) Quantum circuit for readout via nuclear-nuclear two-qubit gates.  $R_{\theta}^{\beta}$  denotes a rotation by an angle  $\theta$  around an axis  $\beta = x, y, z$ . (B) Compilation of the ideal controlled-phase gate using the native nuclear-nuclear interactions.  $U_{-1}(\tau)$  denotes free evolution for a period,  $\tau_{RO} = \pi/8J_{tp}$ , during which time the electron is in the  $m_s = -1$  state. (C) Compilation of (A) using the native interactions. (D) Evolution of the probe spin at the optimal read-out point ( $\tau_{RO} = \pi/8J_{tp}$ ). Orthogonal states of the target spin are mapped into orthogonal states of the probe spin. (E) Characterization curves for all probe-target spin combinations used in this work. The solid lines are a fit to Eq. S24, with resulting fit parameters given in Table S3.

In Fig. S3C we show the compiled readout circuit as implemented in the experiment. Note that this sequence incurs an additional  $\pi$ -rotation to the target spin which we do not rectify, as the state is discarded after the measurement. The unitary evolution describing the full sequence is given by

$$U_{RO} = R_p^x(-\pi/2) \cdot U_{SEDOR}(\tau_{RO}) \cdot R_p^y(\pi/2). \quad (S16)$$

We first initialize the probe spin in the state  $|\uparrow\rangle$ , while the target spin is in an unknown state which is to be read out in the  $\sigma^z$ -basis. The initial state of the system is therefore given by

$$\rho_i = \begin{pmatrix} 1 & 0 \\ 0 & 0 \end{pmatrix} \otimes \begin{pmatrix} a & b \\ c & d \end{pmatrix}, \quad (S17)$$

where  $\langle\sigma_t^z\rangle_i = a - d$  is the expectation value we would like to read out. After applying the nuclear-nuclear readout sequence (Eq. S16), and tracing over the target spin, we find the final state and associated  $\sigma^z$ -basis spin projection of the probe spin as desired, given by

$$\rho_{p,f} = \text{Tr}_t(U_{RO}\rho_f U_{RO}^\dagger) = \begin{pmatrix} a & 0 \\ 0 & d \end{pmatrix}, \quad (S18)$$

$$\langle\sigma_p^z\rangle_f = \text{Tr}(\rho_{p,f}\sigma_p^z) = a - d = \langle\sigma_t^z\rangle_i. \quad (S19)$$

The state of the probe spin can then be read out via the electron spin using previously developed approaches [1, 15]. Importantly, after this measurement, the probe spin can be reinitialized via a swap operation with the electron spin [1, 15], and can then be further used to probe the state of additional target spins. Readout of other bases can be achieved via single-qubit rotations of the target spin prior to the nuclear-nuclear readout sequence.

## B. Quantifying nuclear-nuclear readout in the presence of experimental errors

While the above analysis shows that the readout scheme effectively maps the state of a target spin onto a probe spin via their mutual coupling, the measured signal may be affected by a number of experimental imperfections. These imperfections typically lead to two effects. First, pulse errors on the target spin can cause the readout sequence to fail. Second, the measurement contrast can be reduced due to decoherence of the probe spin or imperfect mapping of the probe spin state to the electron spin. Here we show that we can use the signal obtained via an orthogonal measurement basis to characterize these imperfections and thereby extract the underlying  $\langle \sigma_t^z \rangle_i$ .

In Eq. S16, the final rotation  $R_p^x(-\pi/2)$  maps  $\langle \sigma_p^y \rangle$  to  $\langle \sigma_p^z \rangle$ . If we instead apply a rotation  $R_p^y(-\pi/2)$ , we can measure the expectation value  $\langle \sigma_p^x \rangle$ . We can calculate  $\langle \sigma_p^\phi \rangle_f$  for  $\phi \in \{x, y\}$  as a function of  $\tau$  to get

$$\langle \sigma_p^x \rangle_f(\tau) = \cos(4J_{tp}\tau), \quad (\text{S20})$$

$$\langle \sigma_p^y \rangle_f(\tau) = \langle \sigma_t^z \rangle_i \sin(4J_{tp}\tau). \quad (\text{S21})$$

### 1. Pulse errors on the target spin

First, we consider the effect of pulse errors on the target spin. In particular, we denote a probability,  $\epsilon$ , with which the pulse fails to invert the target. In such cases, the probe spin coherence is preserved by its own inversion pulse, but the target spin is decoupled, turning off the interaction. Thus we have  $\langle \sigma_p^x \rangle = 1$  and  $\langle \sigma_p^y \rangle = 0$ . Taking a statistical average according to the failure rate, we arrive at the expectation values

$$\langle \sigma_p^x \rangle_f(\tau, \epsilon) = \epsilon + (1 - \epsilon) \cos(4J_{tp}\tau), \quad (\text{S22})$$

$$\langle \sigma_p^y \rangle_f(\tau, \epsilon) = (1 - \epsilon) \langle \sigma_t^z \rangle_i \sin(4J_{tp}\tau). \quad (\text{S23})$$

### 2. Amplitude Damping

Second, we consider effects which result in a dampened signal. These include imperfect mapping from the probe spin to the electron spin, pulse errors on the probe spin (resulting in dephasing on a timescale  $T_2^* \ll \tau_{\text{RO}}$ ), and  $T_2$ -timescale dephasing of the probe spin. All of these effects can be encapsulated by a constant factor  $\delta$ , alongside a time-dependent function  $f(t) = \exp[-\tau/\tau_0]^n$ . Here,  $\tau_0$  and  $n$  are the characteristic timescale and exponent for the decay of the signal. Applying these terms to Eqs. S22, S23, we find

$$\langle \sigma_p^x \rangle_f(\tau, \delta, \epsilon, n, \tau_0, \beta) = \delta \exp[-(\tau/\tau_0)^n] (\epsilon + (1 - \epsilon) \cos(4\beta J_{tp}\tau)), \quad (\text{S24})$$

$$\langle \sigma_p^y \rangle_f(\tau, \delta, \epsilon, n, \tau_0, \beta) = \delta \exp[-(\tau/\tau_0)^n] (1 - \epsilon) \langle \sigma_t^z \rangle_i \sin(4\beta J_{tp}\tau). \quad (\text{S25})$$

Here  $\beta$  is a multiplicative factor to account for small changes in coupling frequency due to unwanted couplings to other spins.

### 3. Mitigating experimental imperfections

Considering Eq. S24, we note that the  $\langle \sigma_p^x \rangle_f$  readout signal is dependent on all of the discussed experimental imperfections, but critically does not depend on the initial target spin polarization. Therefore, we can use this signal to characterize those parameters. Fig. S3 shows characterization curves for all probe-target spin combinations used in this work. We fit the data using Eq. S24 and the resulting fit parameters are given in Table S3. Once  $\beta$ ,  $\delta$ ,  $\epsilon$ ,  $\tau_0$ , and  $n$  have been identified, these values can be used to obtain  $\langle \sigma_t^z \rangle_i$  by performing the  $\langle \sigma_p^y \rangle_f$  measurement at  $\tau_{\text{RO}}$  and inverting Eq. S25 to give

$$\langle \sigma_t^z \rangle_i = \frac{\langle \sigma_p^y \rangle_f}{\delta \sin(4\beta J_{tp}\tau_{\text{RO}}) \exp[-(\tau_{\text{RO}}/\tau_0)^n] (1 - \epsilon)}, \quad (\text{S26})$$

## C. Readout for the 1D chain

To read out the spins making up the 1D chain, we use a combination of previously developed electron-nuclear two-qubit gates [1] and our new nuclear-nuclear readout method. The circuits used for initialization and readout via

| Spin | Gate Type | $\tau$ ( $\mu$ s) | $N$ | $C_Q$   | Spin | Probe | $\tau_{\text{RO}}$ (ms) | $\beta$ | $\delta$ | $\epsilon$ | $\tau_0$ (ms) | $n$  |
|------|-----------|-------------------|-----|---------|------|-------|-------------------------|---------|----------|------------|---------------|------|
| 2    | DDrf      | 37.04             | 32  | 0.65(3) | 1    | 2     | 5.76                    | 0.92(1) | 0.52(2)  | 0.09(2)    | -             | -    |
| 5    | DDrf      | 37.04             | 32  | 0.64(3) | 3    | 2     | 14.06                   | 0.90(1) | 0.48(2)  | 0.12(2)    | -             | -    |
| 6    | DD        | 16.48             | 20  | 0.91(1) | 4    | 5     | 25.00                   | 1.06(2) | 0.43(3)  | 0.11(3)    | 65(4)         | 3(1) |
| 8    | DD        | 4.932             | 90  | 0.88(2) | 7    | 8     | 17.86                   | 0.88(1) | 0.57(2)  | 0.04(2)    | -             | -    |
|      |           |                   |     |         | 9    | 8     | 9.89                    | 0.95(1) | 0.57(2)  | 0.09(1)    | -             | -    |

TABLE S3. Readout parameters for the spins in the 1D chain. Left: Readout parameters for the spins that are directly read out using electron-nuclear gates. We use either the DD or DDrf sequence [1], with  $N$  pulses in a CPMG-type sequence with pulse spacing  $\tau$ . Following ref. [1], the parameter  $C_Q$  is measured by initializing the spin in  $|\uparrow\rangle$  and reading out  $\langle\sigma^z\rangle$ , and subsequent measurements are readout corrected so that  $\langle\sigma^z\rangle' = \langle\sigma^z\rangle/C_Q$ . Right: Readout parameters for spins that are read out using the new nuclear-nuclear readout method (section V). The spin state is mapped to a probe spin using a SEDOR sequence with interaction time  $\tau_{\text{RO}}$ . The last five columns give the fit parameters for a characterization measurement using Eq. S24, from which we can estimate  $\langle\sigma^z\rangle$  of the target spin using Eq. S26. Dashed lines indicate spins where no decay was observed on the timescale of the characterization measurement, and therefore the exponential function in Eq. S24 was set to 1.

electron-nuclear two-qubit gates are shown in Fig. 1B of the main text. The compilation of these circuits using native gates is given in Bradley et al. [1]. The method used for readout for each spin, as well as the associated parameters, are given in Table S3. We read out the spins sequentially according to the sequence shown in Fig. 1B of the main text, where the electron spin and any required probe spins are reset before each readout sequence using optical spin pumping and dynamical decoupling based sequences, respectively [1]. Due to the close spectral proximity of spins 3 and 7, which can cause additional errors in the nuclear-nuclear readout sequence, we read out spin 7 in a separate run of the experiment, while the remaining 8 spins are read out sequentially in a single run.

To account for readout imperfections and thereby accurately estimate the expectation values, we correct the results for readout errors using separate characterization measurements. For the spins that are read out directly via the electron spin, we follow the method described in Bradley et al. [1], while for spins that are read out using the nuclear-nuclear readout sequence, we use Eq. S26.

## VI. INITIALIZING THE QUANTUM SIMULATOR: DYNAMIC NUCLEAR POLARIZATION

This section describes the initialization of the spin chain with the PulsePol sequence, a recently developed dynamic nuclear polarization method [16]. We summarize the theoretical background, with a focus on the differences compared to previous studies. We then discuss the optimization of the sequence. In contrast to previous studies, the individual control and measurement enables us to track the polarization dynamics quantitatively and on the single spin level. This reveals that the polarization dynamics themselves present an interesting, and not yet fully understood, many-body problem.

### A. Hamiltonian

Dynamic nuclear polarization (DNP) methods encompass a variety of techniques to realize hyperpolarization of the nuclear spin bath via polarization transfer from a central well-controlled electron spin [16–18]. While the intrinsic energy scales of the differing spin species forbid natural flip-flop interactions between them, the use of Hamiltonian engineering can overcome this barrier. If this process can be made to occur much faster than nuclear spin diffusion, and is combined with fast and high-fidelity electron spin reset, repeated application can lead to large-scale nuclear spin bath polarization [19].

In this work, we employ the recently developed PulsePol sequence which is schematized in Fig. S4A [16]. For values of the characteristic timescale  $\tau$  close to  $\tau_0 \equiv (3\pi/8\gamma_e B_z) = 0.434 \mu\text{s}$ , the effective system Hamiltonian is given by

$$H_{\text{eff}} = \sum_j \Delta\omega_j I_j^z - \sum_j \alpha A_j^\perp (S^+ I_j^- + S^- I_j^+), \quad (\text{S27})$$

where  $\Delta\omega_j \approx [\gamma_e B_z - (A_j^\parallel/2) - (3\pi/8\tau)]$  and  $\alpha = (2/\sqrt{12}\pi) \approx 0.184$ .  $I_j^\pm$  and  $S^\pm$  are spin-1/2 ladder operators for the  $j$ -th nuclear spin and the electron spin respectively (the unoccupied  $m_s = +1$  level is neglected), and the sum is over all the nuclear spins of the environment. Importantly, this Hamiltonian differs from that given in Schwartz et al. [16] by the term  $\sum_j \Delta\omega_j I_j^z$ . This term, arising at first order from the individual hyperfine couplings  $A_j^\parallel$ , introduces  $z$ -disorder between nuclear spins which plays a central role in the polarization transfer process.

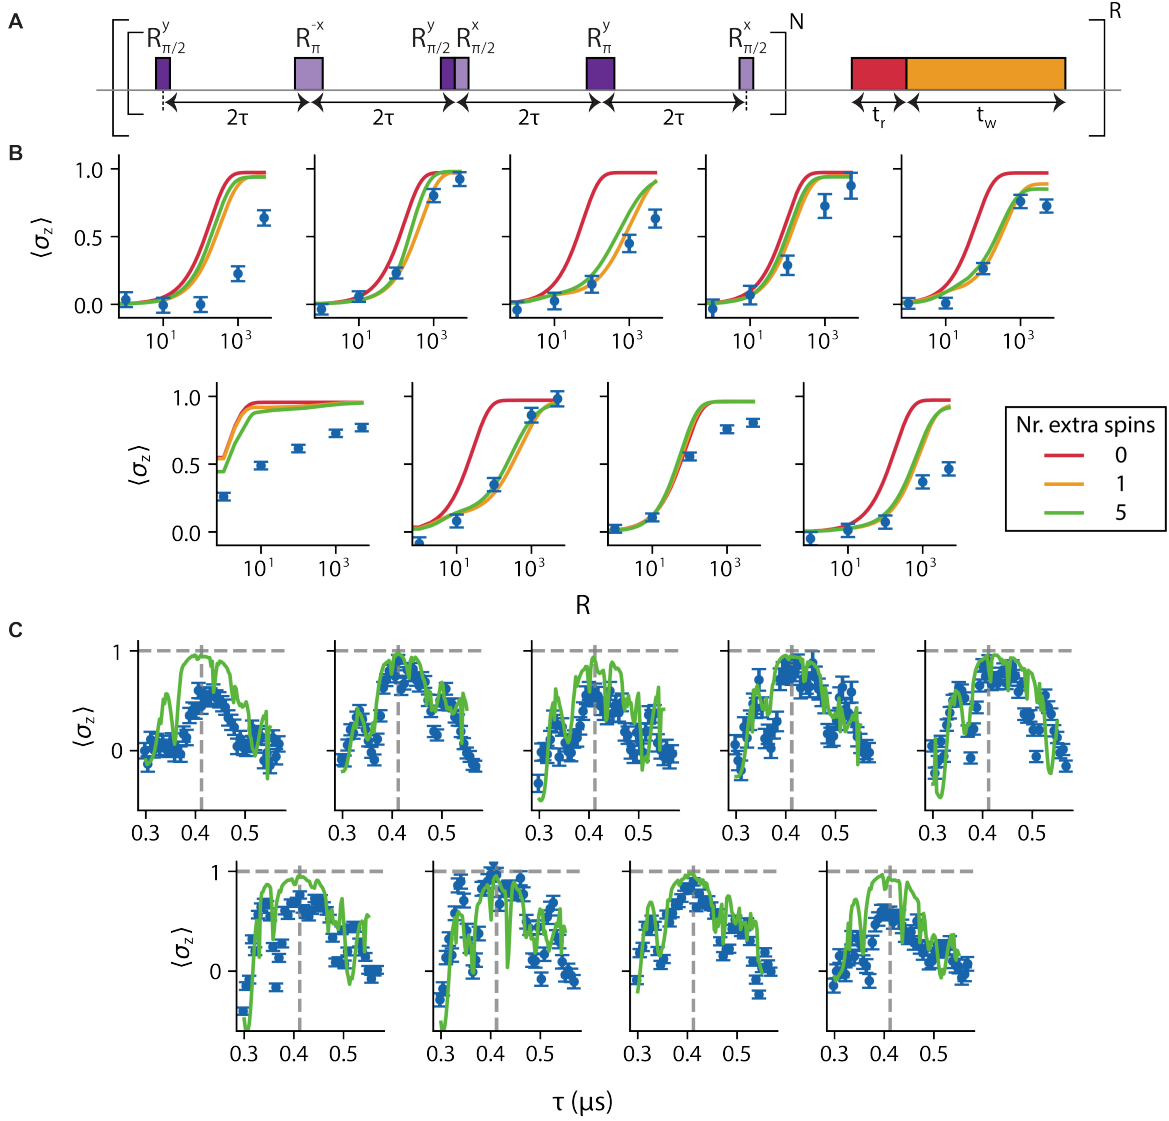

FIG. S4. **PulsePol characterization.** (A) Schematic representation of the PulsePol sequence. The purple pulses are microwave pulses that act on the electron spin.  $t_r = 10 \mu\text{s}$  is the reset time (the total time for which the reset laser is applied) and  $t_w = 14 \mu\text{s}$  is a waiting time that was included due to hardware restrictions. (B) Polarization of each spin (1-9 from top left to bottom right) as a function of the number of repetitions  $R$  for  $\tau = 0.412 \mu\text{s}$  and  $N = 4$ . The red, orange and green solid lines are simulations of the  $^{13}\text{C}$  spin of interest, the  $^{14}\text{N}$  spin, and an additional 0, 1 or 5 spins included in the environment respectively, which were chosen using the method described in the text. (C) Polarization of each spin (1-9 from top left to bottom right) as a function of the parameter  $\tau$  of PulsePol with  $N = 4$  and  $R = 5000$ . Solid lines are the results of simulations including 5 environmental spins. The dashed vertical line represents the value of  $\tau$  employed in the DTC experiments and the horizontal line at a polarization value of 1 is included as a guide to the eye.

As described in Villazon et al. [20], Hamiltonians which do not exhibit z-disorder host dark states which prevent complete polarization of the system, even after an infinite number of DNP cycles. The origin of this z-disorder in our Hamiltonian (in contrast to Ref. [16]) is due to the different choice of electron effective-spin-1/2 basis states. Using the  $m_s = 0$  and  $m_s = -1$  levels (rather than  $m_s = \pm 1/2$ ), the bare system Hamiltonian from which the effective Hamiltonian is derived is

$$H = \sum_j \gamma_c B_z I_j^z - |-1\rangle \langle -1| \sum_j \left( A_j^\perp I_j^x + A_j^\parallel I_j^z \right), \quad (\text{S28})$$

where  $|-1\rangle \langle -1|$  is the projector on the  $m_s = -1$  state of the electron spin.

| Spin | Env. 1 | Env. 2 | Env. 3 | Env. 4 | Env. 5 | Spin | $A_{\parallel}$ (kHz) | $A_{\perp}$ (kHz) |
|------|--------|--------|--------|--------|--------|------|-----------------------|-------------------|
| 1    | 6      | 12     | 13     | 14     | 11     | 10   | 213.154(1)            | 3.0(4)            |
| 2    | 15     | 11     | 12     | 10     | 6      | 11   | -36.308(1)            | 26.62(4)          |
| 3    | 6      | 12     | 13     | 7      | 11     | 12   | 20.569(1)             | 41.51(3)          |
| 4    | 6      | 12     | 13     | 11     | 10     | 13   | 24.399(1)             | 24.81(4)          |
| 5    | 6      | 12     | 13     | 7      | 11     | 14   | 14.548(3)             | 10(1)             |
| 6    | 7      | 12     | 3      | 13     | 11     | 15   | -20.72(1)             | 12(1)             |
| 7    | 6      | 13     | 12     | 11     | 10     | 16   | -4.039(5)             | 0(3)              |
| 8    | 6      | 10     | 12     | 13     | 11     |      |                       |                   |
| 9    | 6      | 12     | 5      | 13     | 11     |      |                       |                   |

TABLE S4. Parameters for the simulations used in Fig. S4. Left: Five most relevant spins (Env. 1-5) for each simulated spin according to Eq. S30. Simulations which incorporated only one environmental spin use Env. 1. Right: Measured parameters for the Spins 10-16 that were employed in the simulations, taken from Abobeih et al. [2] (Spin 16 is used in simulations in section VII).  $A_{\parallel}$  ( $A_{\perp}$ ) is the parallel (perpendicular) hyperfine coupling. The parameters for Spins 1-9 are given in Table S1.

### B. Experimental optimization and numerical simulations

The polarization dynamics under PulsePol are dependent on a number of parameters of the sequence: the characteristic timescale  $\tau$ , the number of applications of the PulsePol primitive between electron resets,  $N$ , and the total number of polarization cycles,  $R$  (see Fig. S4A). Based on preliminary simulations of the system, we identified  $N = 4$  as a suitable working point. In Fig. S4B we show the measured polarization of each nuclear spin in the 9 spin chain as a function of  $R$ , for  $\tau = 0.412 \mu\text{s}$ . We observe that the system polarization continues to increase up to at least  $R = 5000$  iterations of PulsePol, which is the value used throughout the presented experiments. In Fig. S4C we show the dependence of the polarization on  $\tau$ . For this choice of  $R$ , the maximal mean polarization for the 9 spin chain,  $\langle \sigma^z \rangle = 0.75(2)$ , is obtained at  $\tau = 0.412 \mu\text{s}$ , corresponding to an average single-qubit initialization fidelity of  $F_{\text{init}} = 0.88(1)$  (Fig. 1E of the main text). This value of  $\tau$  is detuned from the centre of the expected resonance: at  $\tau_0 \approx 0.436 \mu\text{s}$  we find  $\langle \sigma^z \rangle = 0.64(2)$ . The mechanism behind the reduced polarization rate at the resonant value is not yet well understood, but may arise due to the simultaneous addressing of a larger number of spins in the environment, leading to slower polarization for the targeted spins used in this work.

To explain the observed polarization, we compare the results to numerical simulations for the same conditions, using the Hamiltonian of Eq. S28, and taking into account experimental imperfections. In particular, electron  $\pi$  ( $\pi/2$ ) rotations are modelled by finite square pulses with a duration of 30 ns (15 ns). Furthermore, we account for the finite waiting time of  $\sim 24 \mu\text{s}$  spent in  $m_s = 0$  between the electron reset — which is expected to occur in  $\sim 500$  ns for the 30 nW optical power used here [21] — and the start of the next PulsePol cycle. We further include the nitrogen spin, which adds Hamiltonian terms:

$$H_N = Q(I_N^z)^2 + \gamma_N B_z I_N^z - |-1\rangle \langle -1| \otimes \left( A_N^{\parallel} I_N^z + A_N^{\perp} I_N^x \right), \quad (\text{S29})$$

where  $Q/2\pi = -4.945\text{MHz}$  is the quadrupole splitting,  $\gamma_N$  is the gyromagnetic ratio of the nitrogen,  $A_N^{\parallel}$  ( $A_N^{\perp}$ ) is the parallel (perpendicular) electron-nuclear hyperfine component and  $I_N^{\alpha}$  are the spin-1 matrices for the nitrogen spin.

One challenge is that it is not possible to numerically simulate a large number of spins using exact diagonalization. In the course of investigation through simulations, it became apparent that including particular subsets of the 27 known  $^{13}\text{C}$  spins [2] could lead to vastly different polarization dynamics. In the present approach, for each spin shown in Fig. S4, we first simulate the result when combined pairwise with each of the other known spins. We then select the 5  $^{13}\text{C}$  spins (alongside the target and the nitrogen spin) which have the largest impact, as quantified by

$$\xi_{jk} = \sum_{R=1}^{5000} |\text{PP}_1(j, \tau, N, R) - \text{PP}(j, k, \tau, N, R)|, \quad (\text{S30})$$

where  $\tau$ ,  $N$  and  $R$  are the PulsePol parameters,  $\text{PP}_1(j, \tau, N, R)$  is the polarization of the  $j$ -th  $^{13}\text{C}$  spin after PulsePol without including any other spin in the simulation (red line in Fig. S4B)) and  $\text{PP}(j, k, \tau, N, R)$  is the polarization of the  $j$ -th  $^{13}\text{C}$  spin when including also the  $k$ -th spin (orange line in Fig. S4B).  $\xi_{jk}$  is the integral of the absolute area between the red and orange solid lines in Fig. S4B. These sets of spins, shown in Table S4, are used for the simulations shown in Fig. S4. Typically, spins found to have the largest impact were those with similar  $A^{\parallel}$  to the target, and those with generally large  $A^{\perp}$ . However, a more comprehensive study of these effects is needed to realize a general framework.

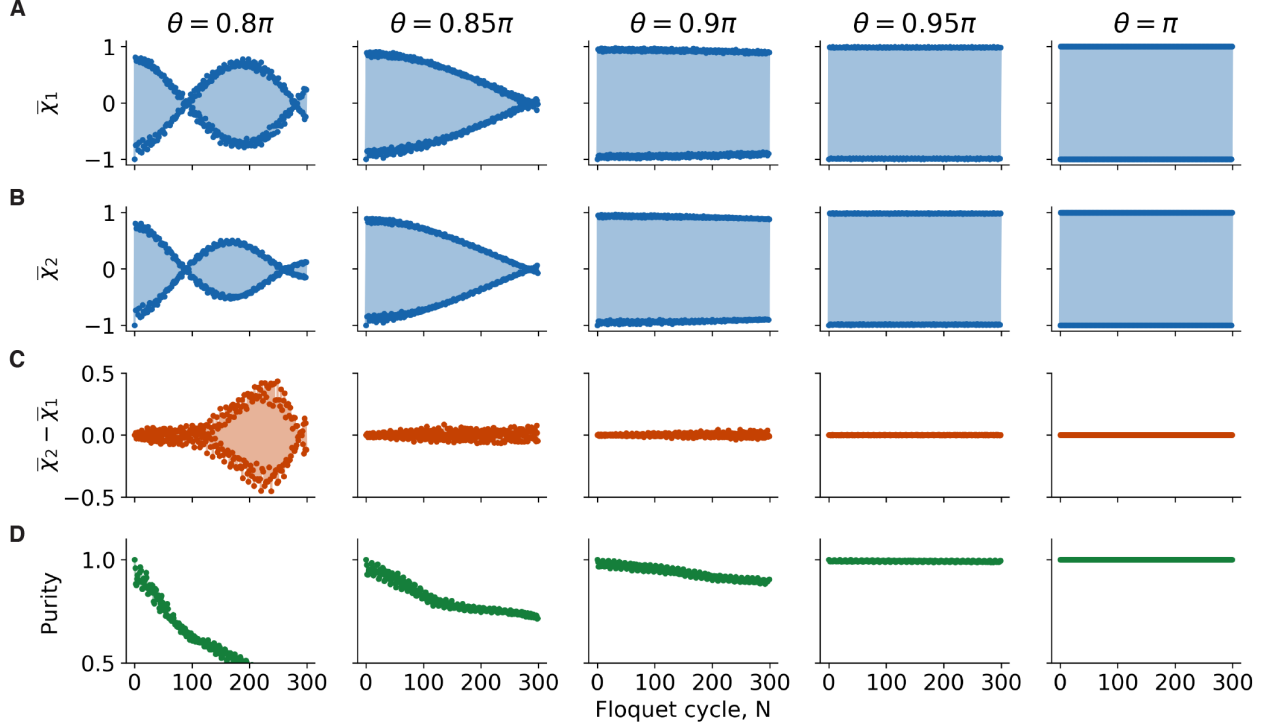

FIG. S5. **Decoherence from the environment.** Numerical simulation of  $U_F$  (section II) showing the averaged two-point correlation  $\bar{\chi}$  as a function of the number of Floquet cycles  $N$  for the first 4 spins of the 1D chain after initializing in the state  $|\uparrow\uparrow\uparrow\uparrow\rangle$ . Columns are for different rotation angles  $\theta$  (indicated at the top) with  $\tau = 5$  ms in all cases. (A) Result with only the 4 targeted spins included in the simulation. (B) Result with 4 additional spins from the environment included (not part of the spin chain, parameters given in Tables S4 and S5). These additional spins are initialized in the maximally mixed state. (C) Difference between the two cases. (D) Purity ( $= \text{Tr}[\rho^2]$ ) of the four-spin reduced density matrix after taking the partial trace over the additional spins.

Despite the inclusion of all of these effects, there remains a discrepancy between the experimentally measured values and the simulation results. While there is reasonable qualitative agreement, the absolute achieved polarization is lower in experiment than that reached in simulation (which is uniformly close to unity). This does not appear to be explained by spin diffusion: the inclusion of a depolarizing channel between resets,  $\Delta_\lambda(\rho) = \lambda\rho + (1 - \lambda)\frac{\mathbf{I}}{\text{Tr}\{\mathbf{I}\}}$ , with  $\lambda = \exp(-8\tau N/T_1)$ , requires a relaxation timescale of 1-10 ms (dependent upon the investigated spin) to induce any noticeable effect. This is at least an order of magnitude shorter than the fastest known relaxation timescales within our system. A second possible cause is the inability to include the full set of known spins in simulation, along with a wider spin bath. The effects of a large number of additional spins are not yet well understood.

Importantly, to our knowledge, our experiment is the first in which DNP techniques have been combined with individual nuclear-spin read-out. Our methods therefore offer new opportunities to study polarization transfer in complex spin systems, and to improve their efficacy.

## VII. DECOHERENCE FROM THE ENVIRONMENT

In this work, we isolate a targeted subset of spins, enabling the realisation of an effective one-dimensional chain in a three-dimensional system. For rotation angles  $\theta \sim \pi$ , we can symmetrize the Floquet sequence to resemble a CPMG sequence in order to simultaneously provide the required decoupling, thereby simplifying the experiment. In Fig. S5, we investigate the effect of the spin environment on the dynamics for different rotation angles. We numerically simulate the Floquet sequence  $U_F$  (section II) up to  $N = 300$  cycles for two cases. First, we include only the first 4 spins of the 1D chain to obtain the ideal dynamics in a perfect closed system. Second, we additionally include 4 spins that are not part of the chain, but couple strongly to the 4 targeted spins (see Table S5 for the parameters of the additional spins). It can be seen that the difference in average two-point correlation between the two cases increases

as  $\theta$  moves away from  $\pi$ . For the value of  $\theta = 0.95\pi$  used in the experiments, the difference remains less than 0.1 over all Floquet cycles simulated. The additional spins can cause shifts in the individual on-site disorder strengths, which can change the measured signal even if the quantum state of the targeted spins remains completely pure. To distinguish these effects, in Fig. S5 we also plot the purity ( $= \text{Tr}[\rho^2]$ ) of the four-spin reduced density matrix after tracing over the additional spins. For  $\theta = 0.95\pi$ , there is a small loss in purity, although this is suppressed compared to larger values of  $\pi - \theta$ . In future experiments, the decoupling pulses and the rotations in the Floquet sequence could be separated so that the rotation angle for the decoupling is always equal to  $\pi$ , allowing lower values of  $\theta$  to be investigated while ensuring good isolation from the spin bath. This would further improve the coherence of the effective 1D chain.

|   | 10        | 11       | 14       | 16       |
|---|-----------|----------|----------|----------|
| 1 | -0.55(2)  | -1.21(1) | -0.23    | 6.34     |
| 2 | -1.885(8) | 0.7(2)   | -0.07    | -3.15(5) |
| 3 | -1.05(8)  | 0.3      | -0.36    | -1.1(2)  |
| 4 | -0.09     | 0.75(2)  | -2.35(2) | 0.05     |

TABLE S5. Interactions between the four targeted spins (1, 2, 3, 4) and the four additional spins included in the simulation (10, 11, 14, 16). Interactions with uncertainties given in parentheses are measured values for the NV electron state  $m_s = -1$ , while interactions shown without uncertainties are calculated from the spin coordinates according to Eq. S13. Hyperfine parameters for the additional spins are given in Table S4.

### VIII. INITIAL STATE DEPENDENCE

In the main text we present the evolution of 11 initial bitstrings, of which 9 are randomly chosen, for up to  $N=300$ -800 Floquet periods. The long-lived subharmonic response observed for all states is consistent with the many-body-localized DTC phase and provides a mechanism to distinguish it from a prethermal response. Here, we present numerical simulations that show clear differences between our system Hamiltonian and a similar Hamiltonian without disorder [10, 12]. These differences manifest themselves within the timescales accessed by our experiments.

We again simulate the Floquet sequence  $U_F$  (section II) for two scenarios, using  $\theta = 0.95\pi$  and  $\tau = 5$  ms. In the first scenario, we use the measured system parameters, with the  $h_j^z$  given by the values of  $A_{\parallel}$  in Table S1, and the  $J_{jk}$  given by the values in Table S2. In the second scenario, we consider the absence of both onsite disorder (all  $h_j^z = 0$ ) as well as the Ising-even disorder terms which can stabilize MBL [10, 12, 22]. That is, we homogenize the  $J_{jk}$  as given in Table S6. We set all the nearest-neighbour couplings equal to the mean magnitude measured across the chain:  $J_0 = 6.67$  Hz, with the remainder of the couplings falling off as a function of distance with an exponent of  $\alpha = 2.5$ .

|   | 1    | 2    | 3    | 4    | 5    | 6    | 7    | 8    | 9    |
|---|------|------|------|------|------|------|------|------|------|
| 1 | -    | 6.67 | 1.18 | 0.43 | 0.21 | 0.12 | 0.07 | 0.05 | 0.04 |
| 2 | 6.67 | -    | 6.67 | 1.18 | 0.43 | 0.21 | 0.12 | 0.07 | 0.05 |
| 3 | 1.18 | 6.67 | -    | 6.67 | 1.18 | 0.43 | 0.21 | 0.12 | 0.07 |
| 4 | 0.43 | 1.18 | 6.67 | -    | 6.67 | 1.18 | 0.43 | 0.21 | 0.12 |
| 5 | 0.21 | 0.43 | 1.18 | 6.67 | -    | 6.67 | 1.18 | 0.43 | 0.21 |
| 6 | 0.12 | 0.21 | 0.43 | 1.18 | 6.67 | -    | 6.67 | 1.18 | 0.43 |
| 7 | 0.07 | 0.12 | 0.21 | 0.43 | 1.18 | 6.67 | -    | 6.67 | 1.18 |
| 8 | 0.05 | 0.07 | 0.12 | 0.21 | 0.43 | 1.18 | 6.67 | -    | 6.67 |
| 9 | 0.04 | 0.05 | 0.07 | 0.12 | 0.21 | 0.43 | 1.18 | 6.67 | -    |

TABLE S6. Pairwise spin-spin interactions  $J_{jk}$  (Hz) for a theoretical homogeneous 9-spin 1D chain, as used for simulations which are free of disorder.

In Figs. S6A,B, we show the simulation results for up to  $N = 10^8$  Floquet periods. Crucially, in the disorder-free case, we see strong variations between differing initial states within  $\sim 100$ -1000 periods. In the presence of disorder, these discrepancies are suppressed up to  $\sim 10^6$  periods. The two scenarios can be distinguished within the experimentally accessed timescales ( $N = 300$ -800 periods, Figs. S6C,D). While we do observe some state-dependence at late times even in the disordered scenario, this is attributed to finite-size effects [10, 23]. Extending to larger system

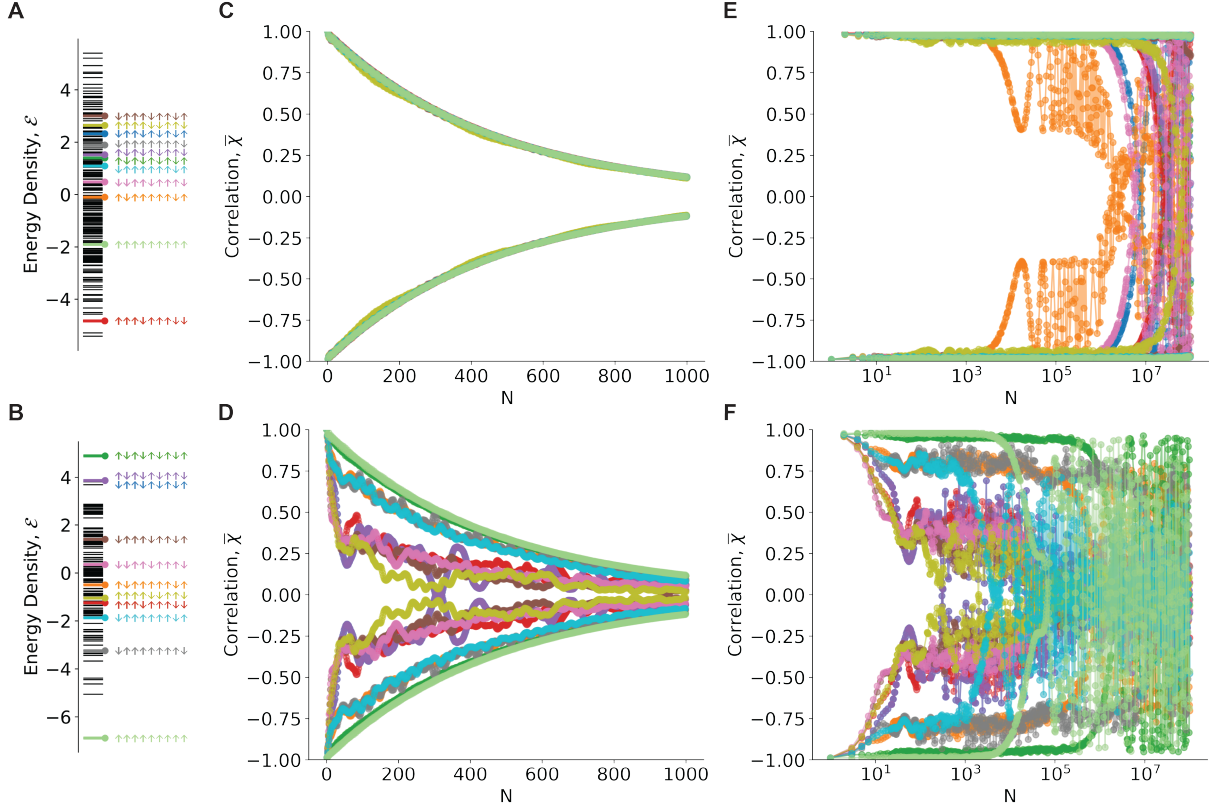

FIG. S6. **Initial state dependence** (A and B) Calculated energy densities  $\varepsilon$  for all possible states of the form  $\bigotimes_j^L |m_j\rangle$ ,  $m_j \in \{\uparrow, \downarrow\}$  (black lines), for the disordered experimental Hamiltonian (Table S2, A) and a theoretical disorder-free Hamiltonian (Table S6, B). The initial states measured in Fig. 4D of the main text are indicated by the corresponding colors. (C and D) Simulated values of the correlation function  $\bar{\chi}$  for the 11 initial states used in the main text experiments, up to  $N = 1000$  Floquet periods, with (C) and without (D) disorder. The simulated results are multiplied by the decay function  $f(N) = Ae^{-N/N_{1/e}}$ , with  $N_{1/e} = 472(17)$  extracted from a fit to the experimental data (Fig. 4D). Clear behavioural differences can be observed within the experimentally accessed timescales. (E and F) Simulated values of the correlation function  $\bar{\chi}$  up to  $N = 10^8$  Floquet periods, with (E) and without (F) disorder.

sizes is expected to stabilize the DTC phase for all bitstrings at increasingly larger times.

- 
- [1] C. E. Bradley, J. Randall, M. H. Abobeih, R. C. Berrevoets, M. J. Degen, M. A. Bakker, M. Markham, D. J. Twitchen, and T. H. Taminiau, *Phys. Rev. X* **9**, 031045 (2019).
  - [2] M. H. Abobeih, J. Randall, C. E. Bradley, H. P. Bartling, M. A. Bakker, M. J. Degen, M. Markham, D. J. Twitchen, and T. H. Taminiau, *Nature* **576**, 411 (2019).
  - [3] M. H. Abobeih, J. Cramer, M. A. Bakker, N. Kalb, M. Markham, D. J. Twitchen, and T. H. Taminiau, *Nat. Commun.* **9**, 2552 (2018).
  - [4] L. Robledo, L. Childress, H. Bernien, B. Hensen, P. F. A. Alkemade, and R. Hanson, *Nature* **477**, 574 (2011).
  - [5] L. M. K. Vandersypen and I. L. Chuang, *Rev. Mod. Phys.* **76**, 1037 (2005).
  - [6] W. S. Warren, *J. Chem. Phys.* **81**, 5437 (1984).
  - [7] T. Gullion, D. B. Baker, and M. S. Conradi, *J. Magn. Reson.* **89**, 479 (1990).
  - [8] T. H. Taminiau, J. J. T. Wagenaar, T. van der Sar, F. Jelezko, V. V. Dobrovitski, and R. Hanson, *Phys. Rev. Lett.* **109**, 137602 (2012).
  - [9] J. R. Johansson, P. D. Nation, and F. Nori, *Comput. Phys. Commun.* **184**, 1234 (2013).
  - [10] V. Khemani, R. Moessner, and S. L. Sondhi, *arXiv preprint arXiv:1910.10745* (2019).
  - [11] F. Machado, D. V. Else, G. D. Kahanamoku-Meyer, C. Nayak, and N. Y. Yao, *Phys. Rev. X* **10**, 011043 (2020).
  - [12] M. Ippoliti, K. Kechedzhi, R. Moessner, S. L. Sondhi, and V. Khemani, *arXiv preprint arXiv:2007.11602* (2020).
  - [13] A. L. Burin, *Phys. Rev. B* **91**, 094202 (2015).

- [14] C. P. Slichter, *Principles of magnetic resonance*, Vol. 1 (Springer Science & Business Media, 2013).
- [15] T. H. Taminiau, J. Cramer, T. van der Sar, V. V. Dobrovitski, and R. Hanson, *Nat. Nanotechnol.* **9**, 171 (2014).
- [16] I. Schwartz, J. Scheuer, B. Tratzmiller, S. Müller, Q. Chen, I. Dhand, Z.-Y. Wang, C. Müller, B. Naydenov, F. Jelezko, *et al.*, *Sci. Adv.* **4**, eaat8978 (2018).
- [17] P. London, J. Scheuer, J.-M. Cai, I. Schwarz, A. Retzker, M. B. Plenio, M. Katagiri, T. Teraji, S. Koizumi, J. Isoya, *et al.*, *Phys. Rev. Lett.* **111**, 067601 (2013).
- [18] J. E. Lang, D. A. Broadway, G. A. L. White, L. T. Hall, A. Stacey, L. C. L. Hollenberg, T. S. Monteiro, and J.-P. Tetienne, *Phys. Rev. Lett.* **123**, 210401 (2019).
- [19] T. Unden, N. Tomek, T. Weggler, F. Frank, P. London, J. Zopes, C. Degen, N. Raatz, J. Meijer, H. Watanabe, *et al.*, *NPJ Quantum Inf.* **4**, 39 (2018).
- [20] T. Villazon, A. Chandran, and P. W. Claeys, *Phys. Rev. Res.* **2**, 032052 (2020), arXiv: 2001.10008.
- [21] A. Reiserer, N. Kalb, M. S. Blok, K. J. M. van Bemmelen, T. H. Taminiau, R. Hanson, D. J. Twitchen, and M. Markham, *Phys. Rev. X* **6**, 021040 (2016).
- [22] N. Y. Yao, A. C. Potter, I.-D. Potirniche, and A. Vishwanath, *Phys. Rev. Lett.* **118**, 030401 (2017).
- [23] D. V. Else, B. Bauer, and C. Nayak, *Phys. Rev. Lett.* **117**, 090402 (2016).
